# Supplementary material for: BIV-Priv-Seg: Locating Private Content in Images Taken by People With Visual Impairments
Source: arXiv:2407.18243 source file (2025-01-10)
Supplement: Supplementary file 1 [file 06-Supplementary_Materials.tex]

\paragraph{Table of contents:}
\begin{itemize}
    \item \textbf{Section 1:} Private Object Categories
    \item \textbf{Section 2:} Annotation Collection Workflow
    \item \textbf{Section 3:} Data Analysis on Paper-Based and Non-Paper-Based Categories
    \item \textbf{Section 4:} Evaluation Results of Mask Level Privacy Classification
    \item \textbf{Section 5:} Qualitative Results of VLM Benchmarked on BIV-Priv-Seg
\end{itemize}

\section{Private Object Categories}

The $16$ categories in our dataset include $14$ categories adopted from previous work~\cite{sharma2023disability} and $2$ additional categories, \emph{pregnancy test box} and \emph{condom packet}. These categories are to complement \emph{pregnancy test} and \emph{condom box} in the previous work~\cite{sharma2023disability} since sometimes the pregnancy tests and condoms were photographed outside the carton boxes while other times they were not.  Consequently, we differentiate the contents inside a box from the box itself.   We also replaced the category \emph{tattoo} with \emph{tattoo sleeve}.  This is because of the technical difficulties of annotating tattoo patterns on tattoo sleeves that individuals wore to mimic tattoos; the definition of the area/range of a tattoo pattern is often vague.  We instead leverage \emph{tattoo sleeve}, which we define as the sleeve object itself that includes the clothing area where tattoo patterns may be absent.\footnote{In the annotation interface, these special categories are provided with more detailed instructions to prevent confusion in the definition of the categories.}

We note that the category ``receipt" already exists in the 100 categories in VizWiz-FewShot. Even though it is indicated in~\cite{sharma2023disability} that bills and receipts are considered private objects for BLV, we preserve both categories in VizWiz-FewShot and BIV-Priv-Seg as both are valuable data in the field. We conducted data post-processing to remove the category in BIV-Priv-Seg before model benchmarking to support the validity of our experiments.

\section{Annotation Collection Workflow}
For the annotation collection of BIV-Priv-Seg, we adopted the methods proposed in previous work~\cite{tseng2022vizwiz}. For a comprehensive quality control, we use the two-annotation quality control approach.  An overview of the workflow is illustrated in \textbf{Figure~\ref{fig:2_ann_quality_control_workflow}}.

\begin{figure}[t!]
\centering
	\includegraphics[width=0.99\linewidth]{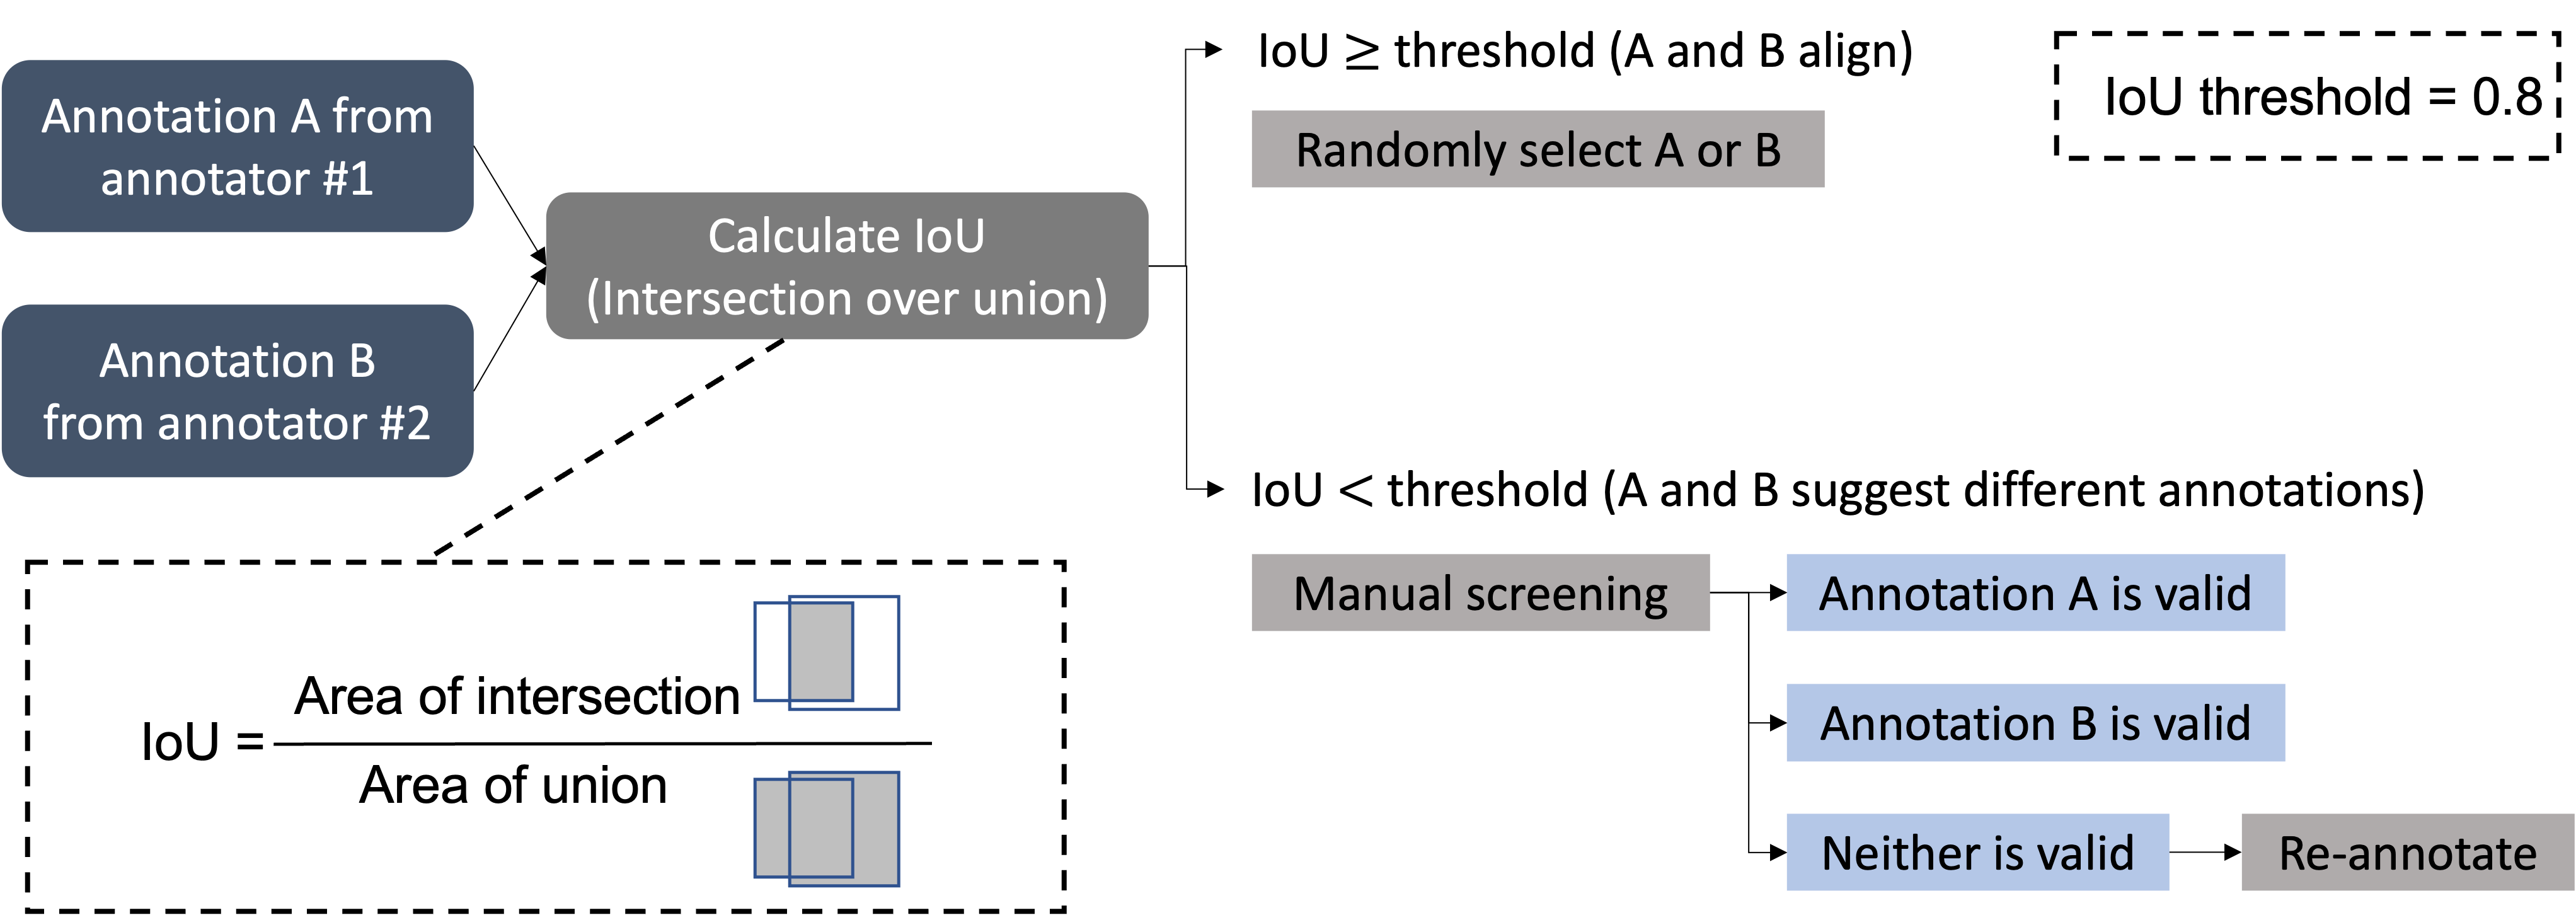} \hfill 
  \caption{Overview of quality control workflow for generating ground truth instance segmentations using the two instance segmentations collected per object.}
  \label{fig:2_ann_quality_control_workflow}
\end{figure}

For the private categories in our dataset, we excluded the additional step of classifying segmented object categories proposed in~\cite{tseng2022vizwiz},  since the number of categories is relatively smaller, at only $16$ category types. In VizWiz-FewShot~\cite{tseng2022vizwiz}, the $100$ categories were separated into $20$ categories per batch through the classification task to ensure the quality of the segmentation task.

\begin{figure}[b!]
\centering
	\includegraphics[width=.48\textwidth]{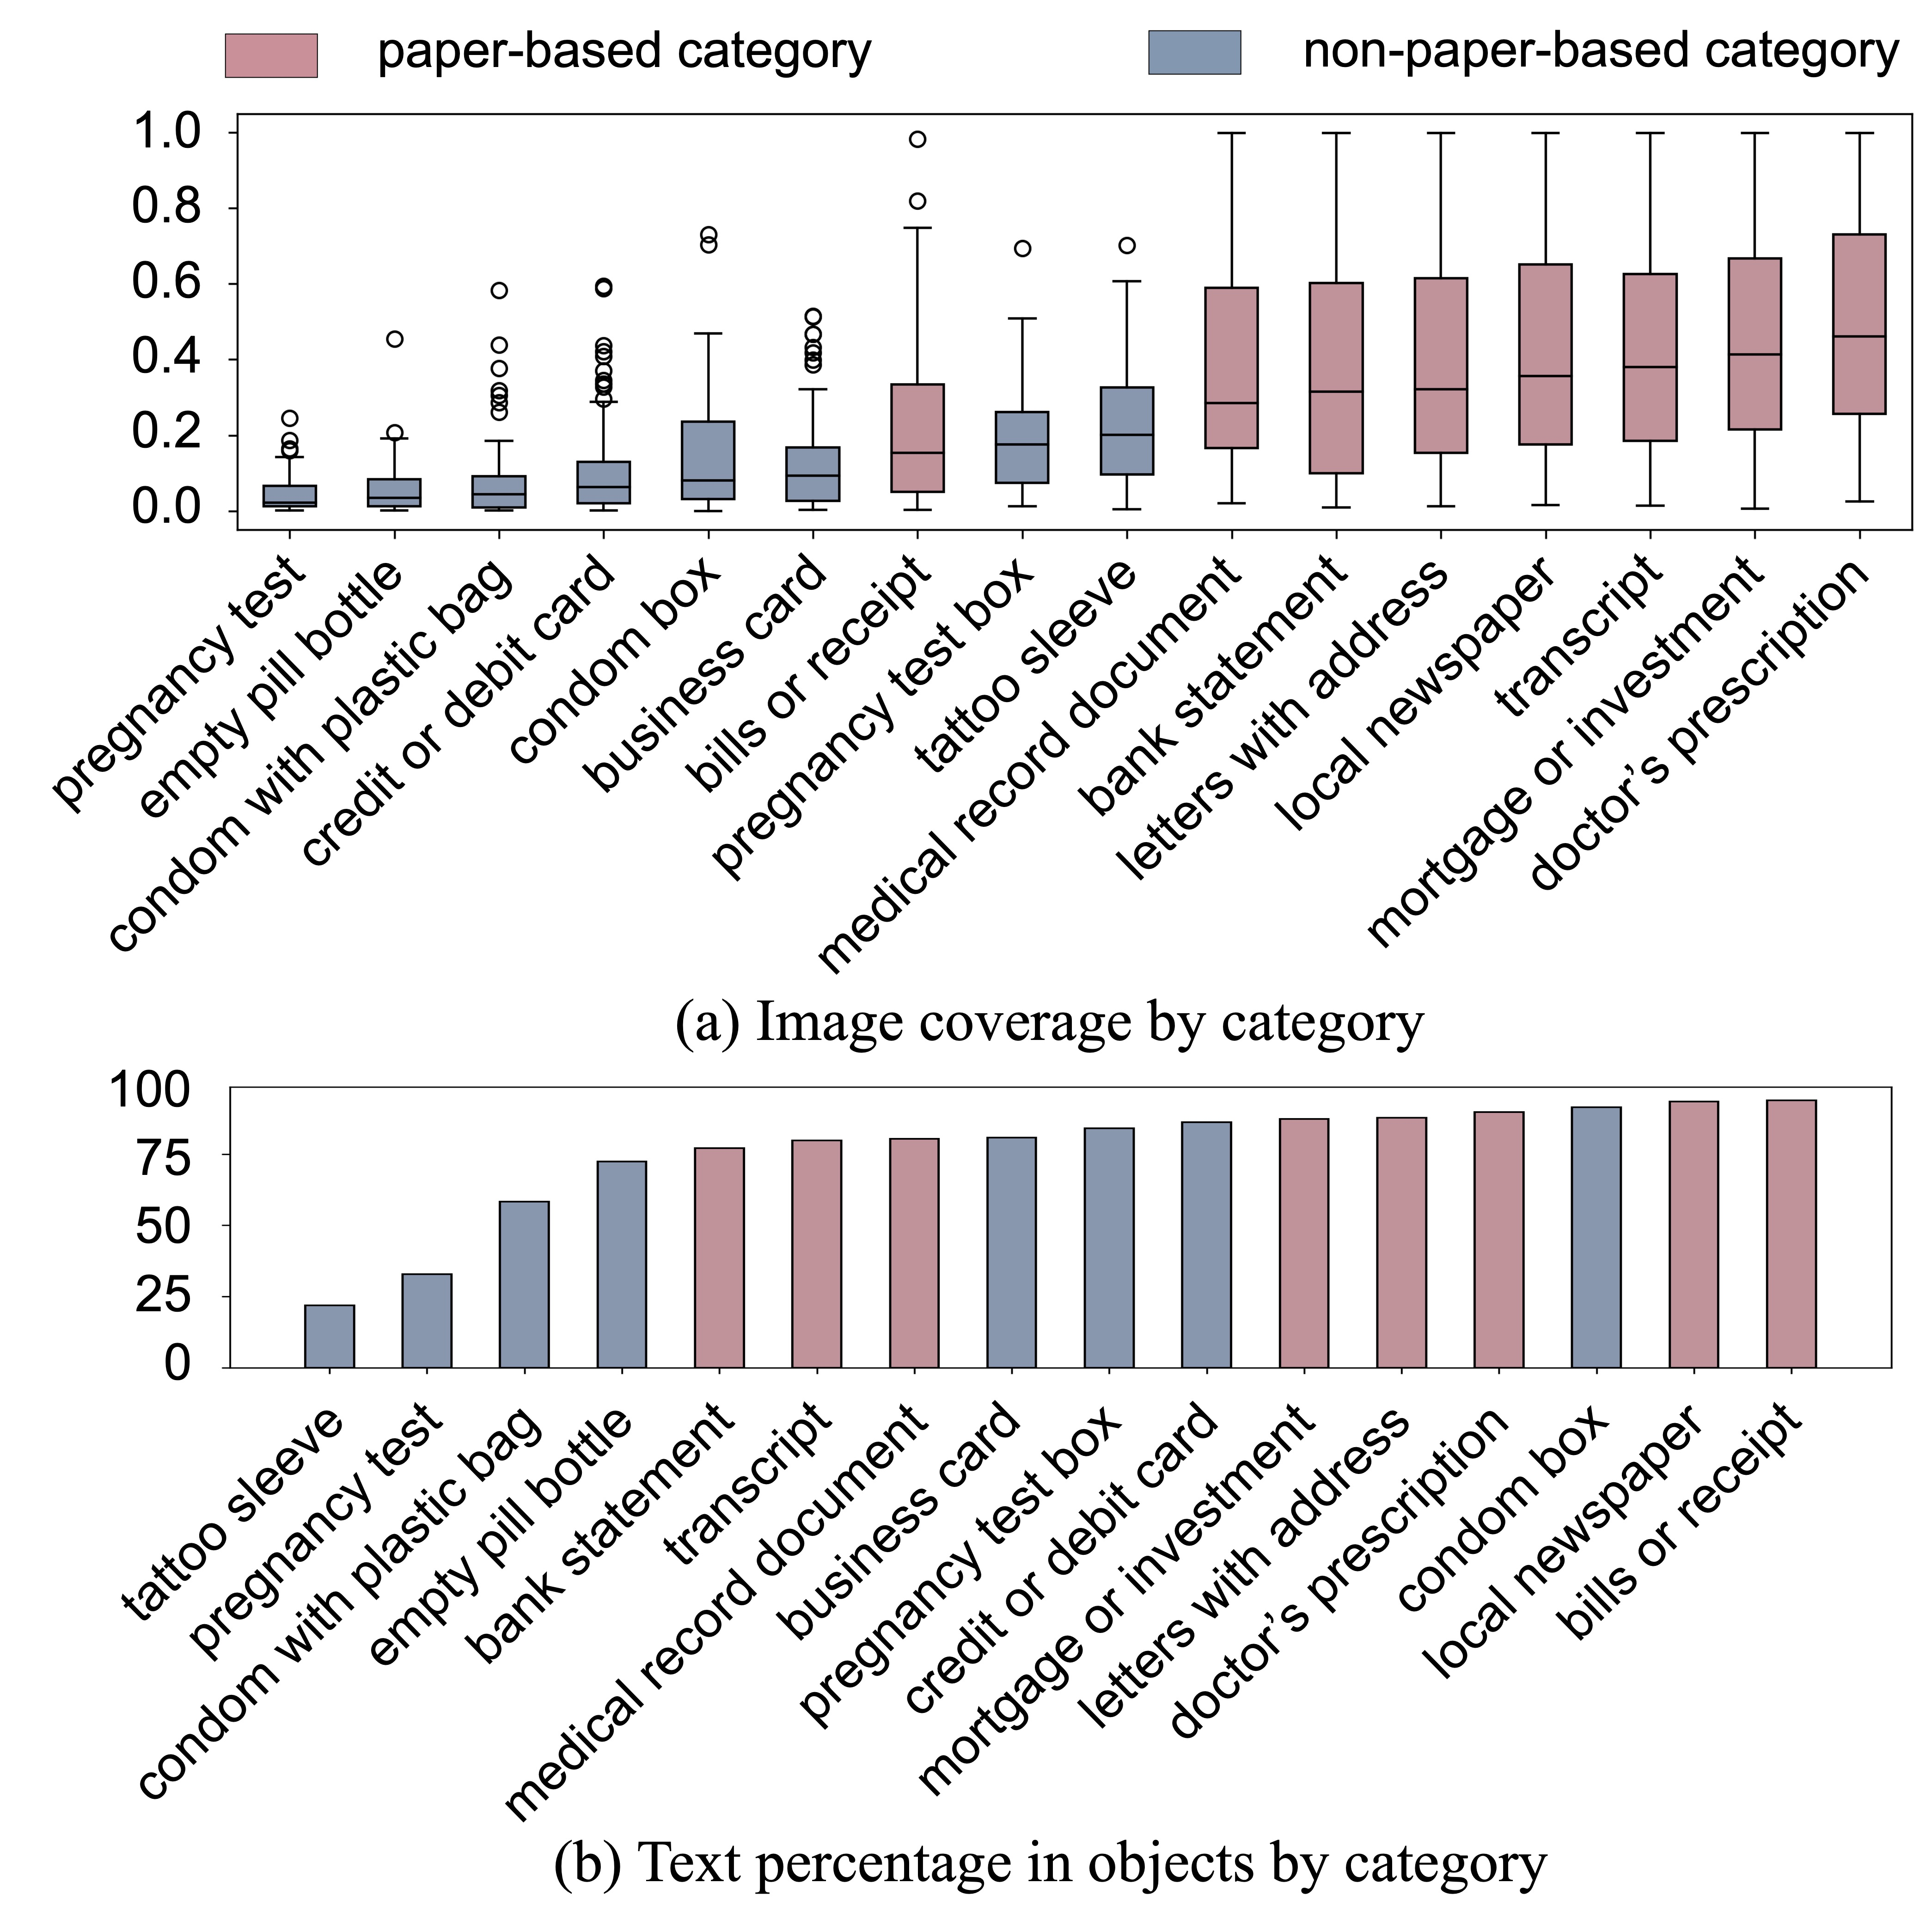} \hfill 
  \vspace{-1.5em}
  \caption{Results of category-based dataset analyses on BIV-Priv-Seg. The plots show (a) the proportion of instances with text sorted by frequency of text for some of the categories and (b) the distribution of image coverage sorted by the medians of the distributions.}   
  \label{fig:category_based_hists}
\end{figure}

\section{Data Analysis on Paper-Based and Non-Paper-Based Categories}
\textbf{Figure~\ref{fig:category_based_hists}(a)} illustrates the image coverage distribution of each category in our dataset. We hypothesize that it is more challenging for the BLV group to adjust the camera to a proper distance from an A4 or letter-sized paper resulting in many paper-based categories tending to have higher image coverage than non-paper-based objects.

\begin{figure}[b!]
\centering
\includegraphics[width=0.48\textwidth]{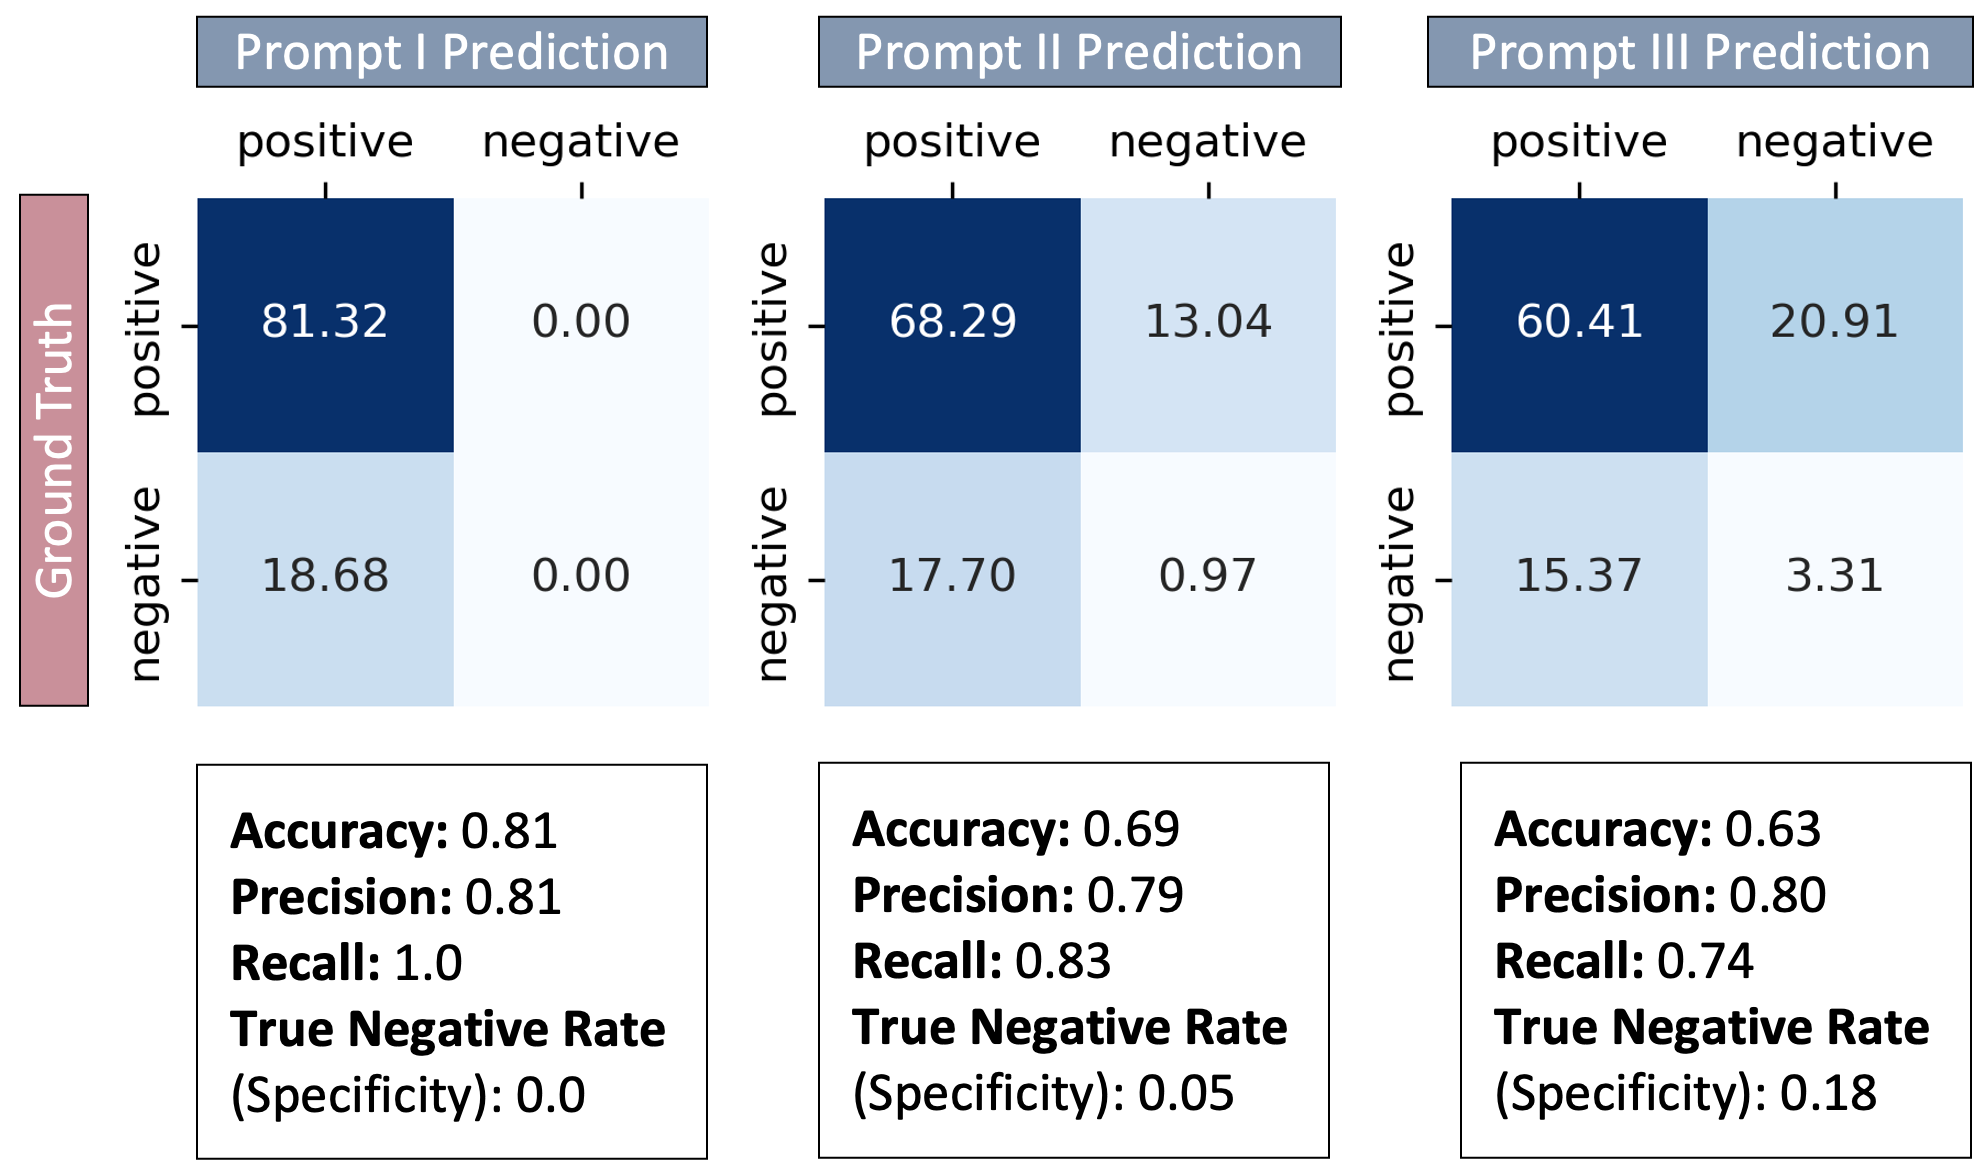}
\caption{GLaMM privacy classification results of prompts I, II, and III on BIV-Priv-Seg in binary classification metrics. The confusion matrices (TP, FP, TN, and FN) are presented in percentages.}
\label{fig:prompts_CM}
\end{figure}

\section{Evaluation Results of Mask Level Privacy Classification}

The detailed evaluation of the GLaMM privacy classification results is presented and analyzed in the section. First, we show the classification results at the \emph{mask level} for the three prompts in \textbf{Figure~\ref{fig:prompts_CM}}. While prompt I achieves the highest accuracy, it does not accurately reflect the model's classification capability since all samples in the dataset are classified as private. Across all tested prompts, it is evident that the model struggles to correctly identify negative samples, meaning no target object is present.

\begin{figure*}[h]
\centering
\includegraphics[width=0.89\textwidth]{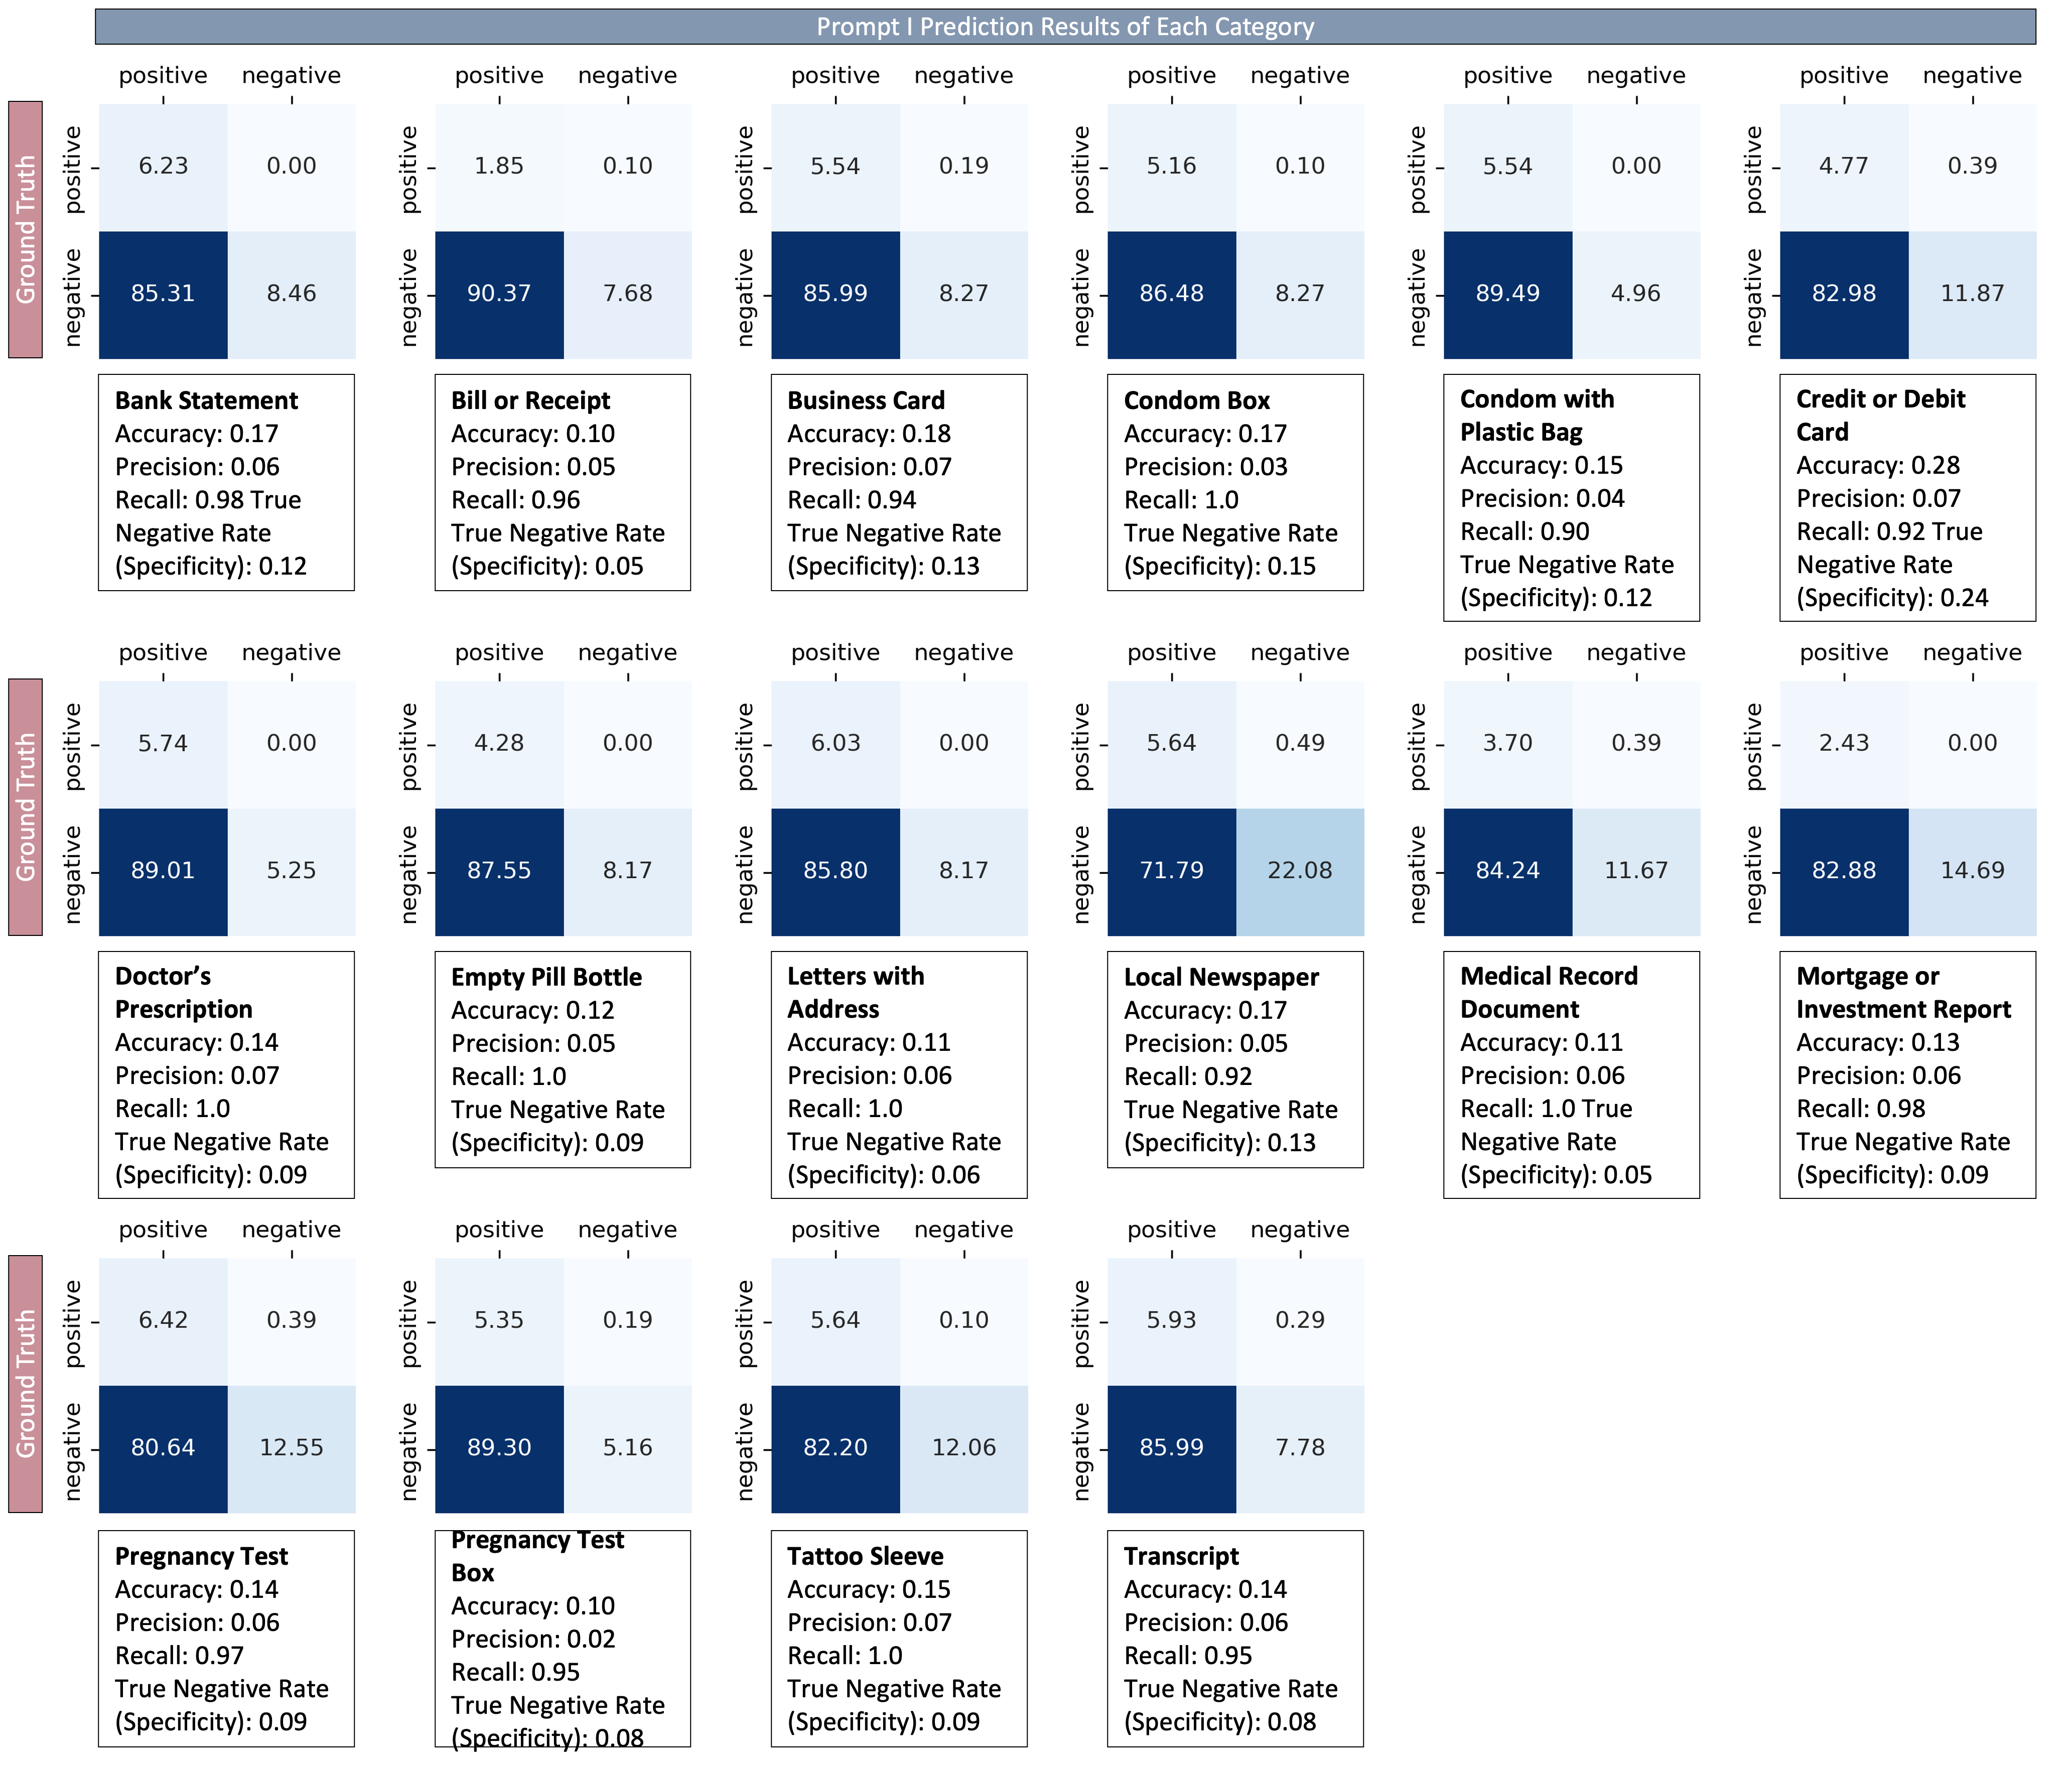}
\caption{GLaMM privacy classification results of prompts I, II, and III on BIV-Priv-Seg in binary classification metrics. The confusion matrices (TP, FP, TN, and FN) are presented in percentages.}
\label{fig:prompt_I_category_CM}
\end{figure*}

Breaking down the 16 categories prompted separately in the prompt I scenario (category-specific scenario), we present the mask-level results of the multi-class classification, including metrics such as confusion matrices in \textbf{Figure~\ref{fig:prompt_I_category_CM}}. The observations align with those from the binary privacy classification: there are generally high recall scores and low true negative (TN) rates. This suggests that while the model has a strong ability to identify positive samples, it struggles significantly with identifying negative samples.

\section{Qualitative Results of VLM Benchmarked on BIV-Priv-Seg}

\textbf{Figure~\ref{fig:gpt_qualitative}} shows qualitative examples of GPT-4o coupled with Dall-E2 with the prompt \emph{``Generate a binary mask that segments the \{category name\}."}. The model failed to generate binary masks for segmentation. \textbf{Figure~\ref{fig:cogvlm_qualitative}} shows qualitative examples CogVLM with prompts I. The model performs poorly by achieving a mAP score at 0.

\begin{figure}[h]
\centering
\includegraphics[width=0.48\textwidth]{images/qualitative_gpt4o Large.jpeg}
\caption{Qualitative results of GPT-4o coupled with Dall-E2~\cite{ramesh2022hierarchical} on BIV-Priv-Seg.}
\label{fig:gpt_qualitative}
\end{figure}

\begin{figure}[h]
\centering
\includegraphics[width=0.48\textwidth]{images/qualitative_cogvlm Large.jpeg}
\caption{Qualitative results of CogVLM~\cite{wang2023cogvlm} on BIV-Priv-Seg.}
\label{fig:cogvlm_qualitative}
\end{figure}

\textbf{Figure~\ref{fig:glamm_prompts_qualitative}} visualizes the examples of prediction results of GLaMM on our dataset. We compare the predictions of prompt I, prompt II, and prompt III to ground truth. Shown are examples of both images with accurate and inaccurate segmentation results from prompt I. In the examples of accurate predictions 
from prompt I, prompt II and prompt III, results often struggle to well-segment the private object. However, in examples such as the bank statement and the pregnancy test in \textbf{Figure~\ref{fig:glamm_prompts_qualitative}}, the explanation of private object leads prompt III to perform better than prompt II.

\begin{figure*}[h]
\centering
\includegraphics[width=0.9\textwidth]{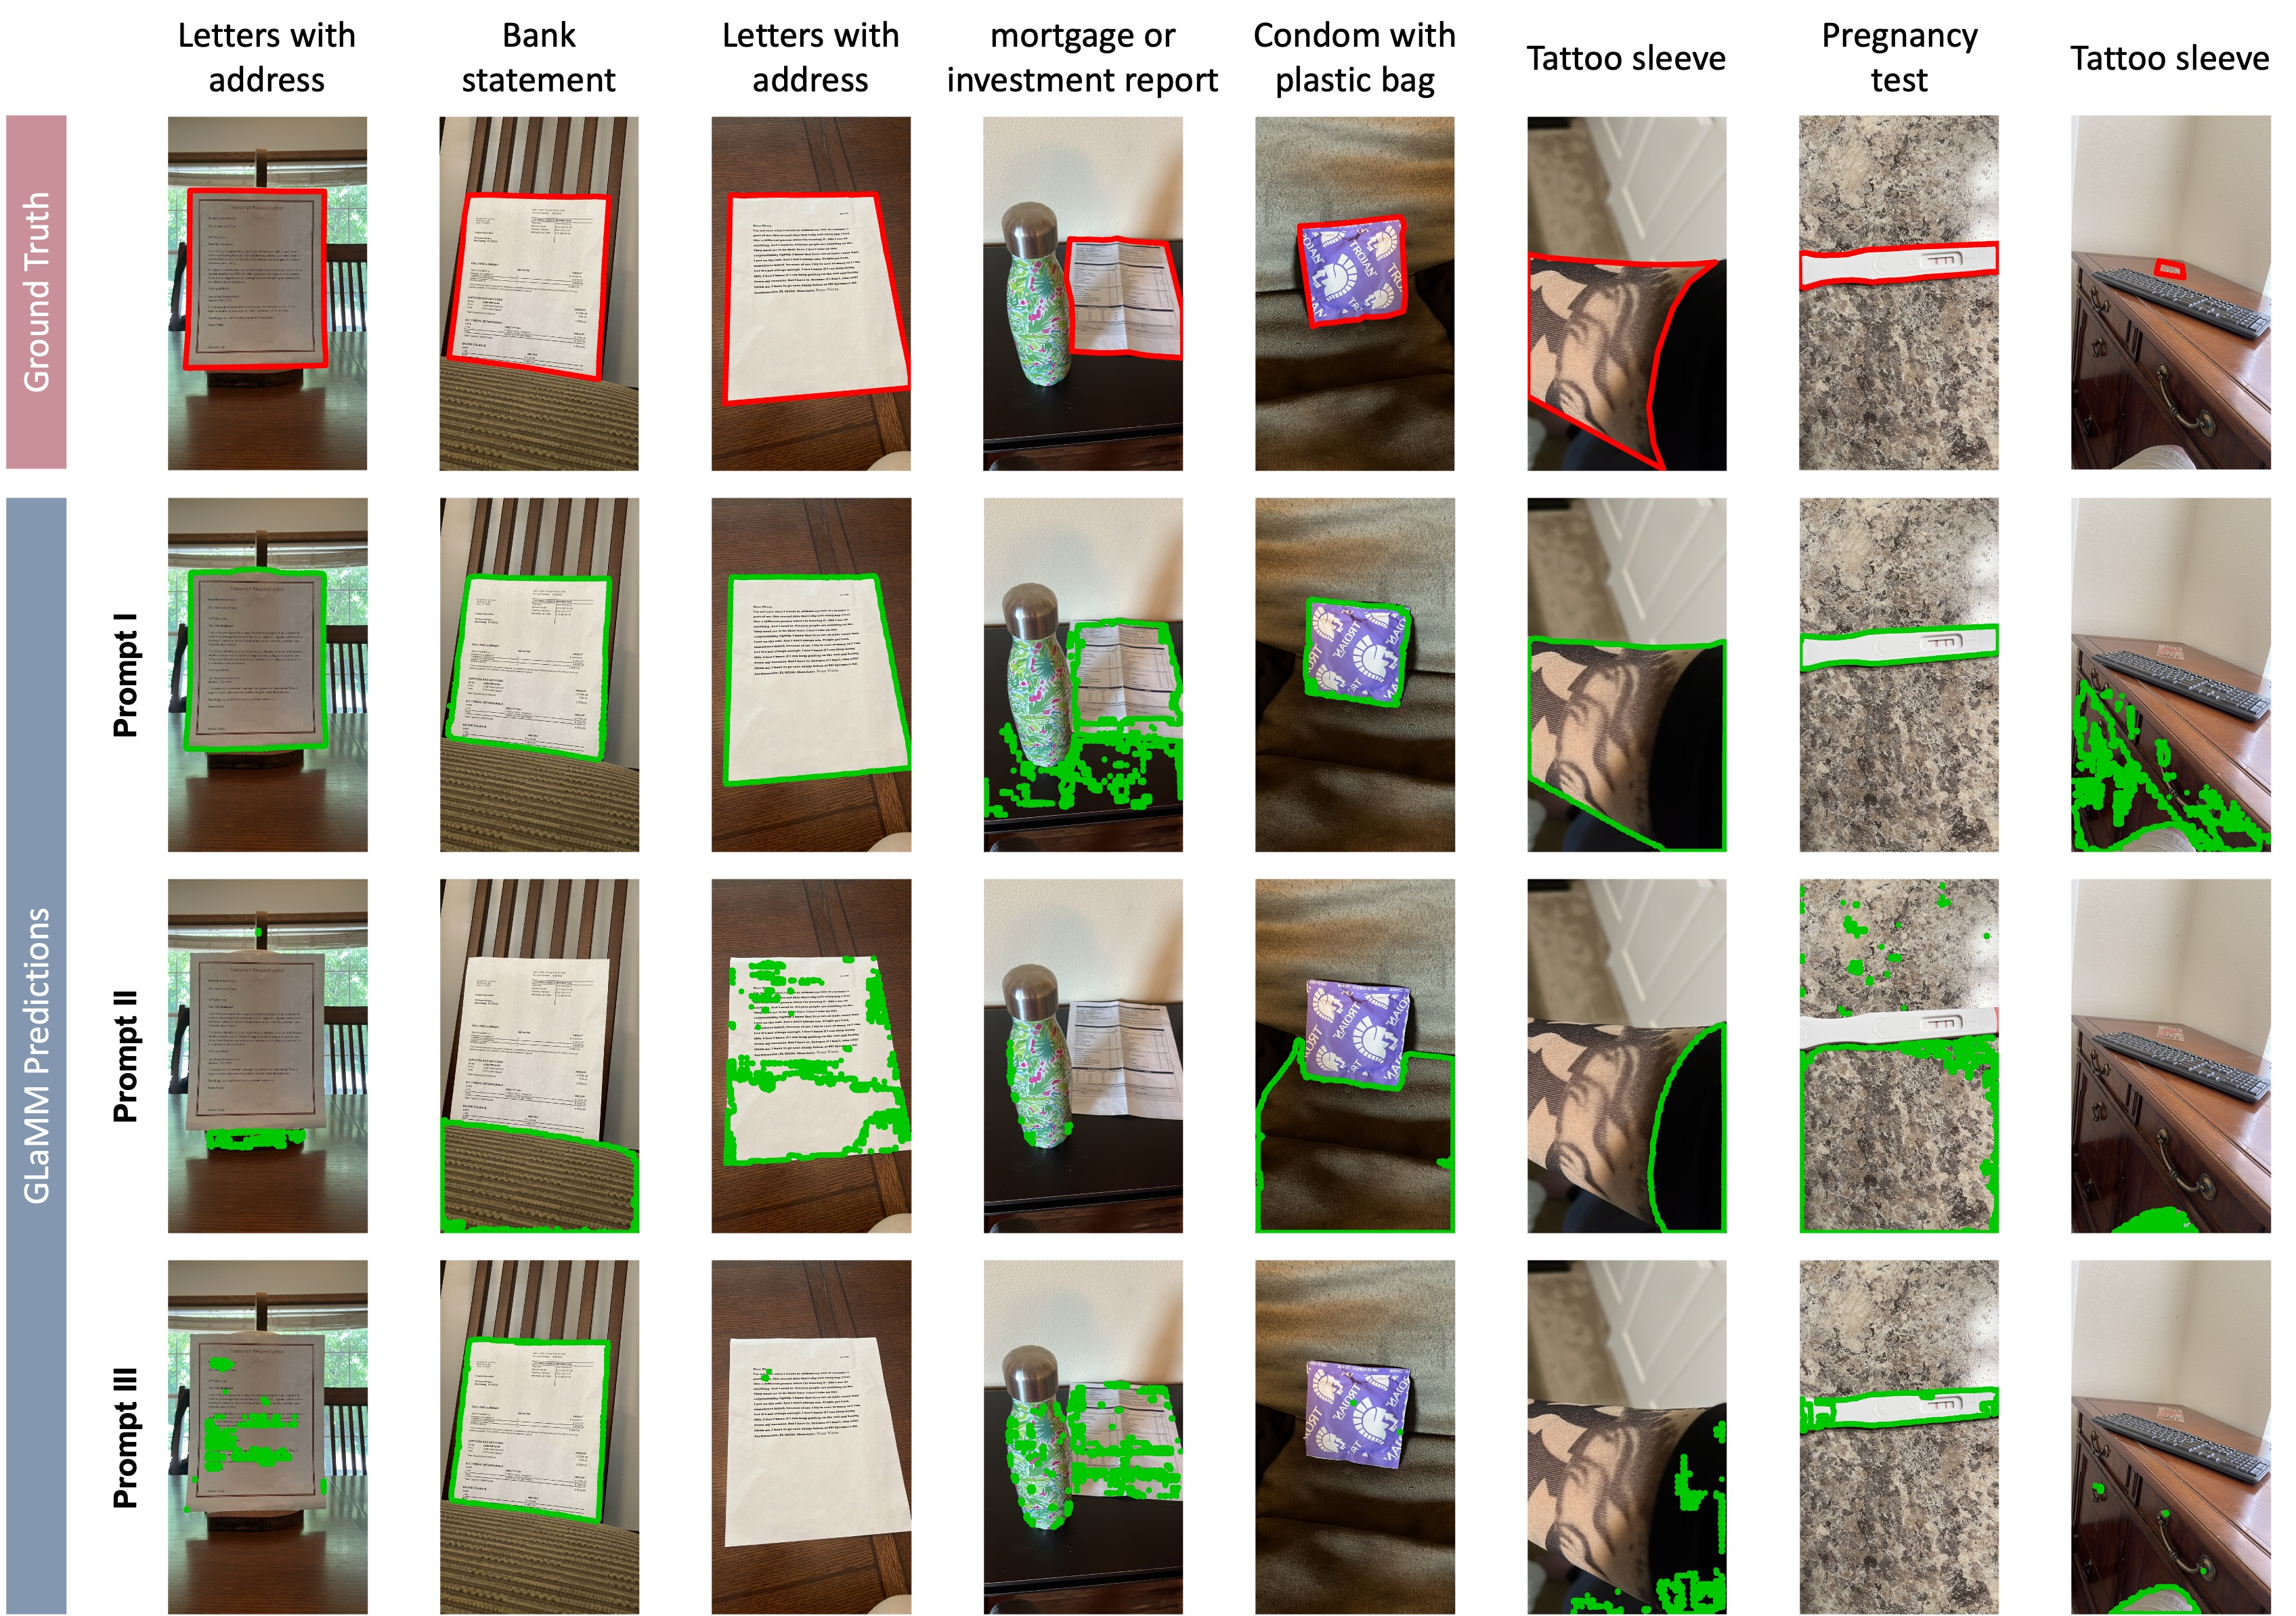}
\caption{Qualitative results of GLaMM on BIV-Priv-Seg.}
\label{fig:glamm_prompts_qualitative}
\end{figure*}

Following the implementation source\footnote{https://github.com/luca-medeiros/lang-segment-anything}, we benchmarked the model of GroundingDINO~\cite{liu2023grounding} coupled with SAM~\cite{kirillov2023segment} on our dataset. \textbf{Figure~\ref{fig:langSAM_qualitative}} visualizes examples of prediction results. Two prompts are used: (1) \emph{``\{category name\}"} and (2) \emph{``private object"}. Results show a similar trend as those of GlaMM, where the model performs better when given the exact category name, while struggling with the more vague notion of ``private object".

\begin{figure}[h]
\centering
\includegraphics[width=0.48\textwidth]{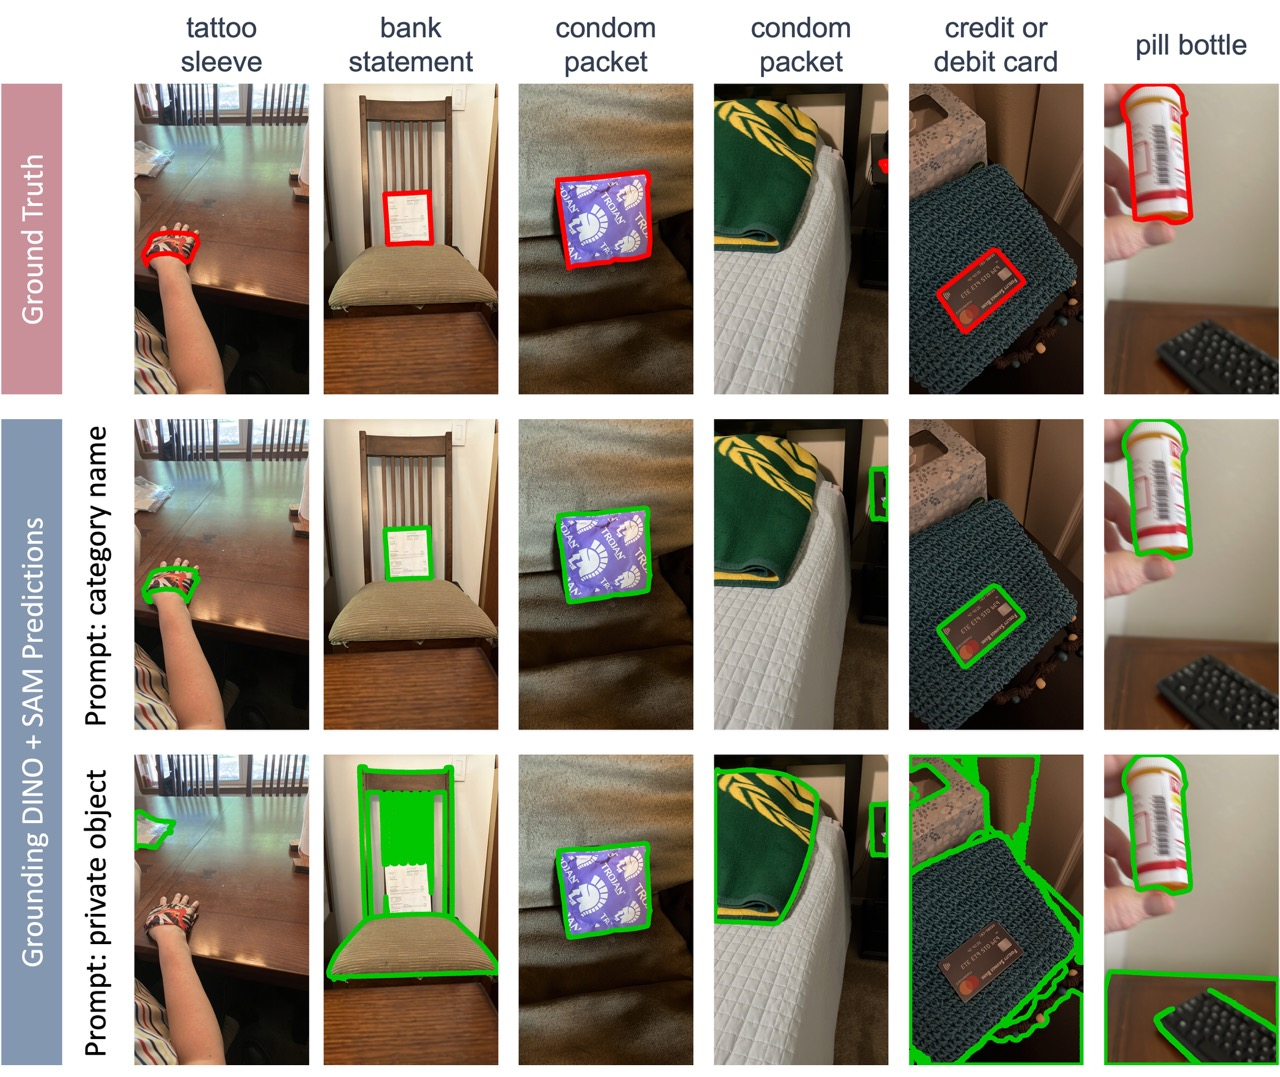}
\caption{Qualitative results of GroundingDINO~\cite{liu2023grounding} coupled with SAM~\cite{kirillov2023segment} on BIV-Priv-Seg.}
\label{fig:langSAM_qualitative}
\end{figure}

% \section{Correlation of Object Saliency and VLM Performance} \label{supp:saliency_and_VLM}

% [TODO] correlation metrics and a plot

% [TODO] qualitative results (showing segmentation examples of salient and non-salient images)
